# Supplementary material for: Dialog state tracking, a machine reading approach using Memory Network
Source: arXiv:1606.04052 source file (2017-03-02)
Supplement: Supplementary file 1 [file appendix.tex]

\newpage
\section{Appendix}

\begin{table}[ht!]
\centering
\caption{{\bf One supporting fact task} : A machine reading task formulated dialog state tracking learning example for the {\it Food} slot from {\it DSTC2} dataset}
\begin{tabular}{|l|l|l|}
\hline\hline
{\bf Index} & {\bf Actor} & {\bf Utterance} \\
\hline
1 & Cust &West part of town cuban food.  \\
2 & Agent &Sorry there is no cuban restaurant in the west of town.  \\
3 & Cust &Ok, do you have an Italian place ?  \\
4 & Agent &Prezzo is a nice restaurant in the west of town serving italian food.  \\
5 & Cust &Phone number.  \\
6 & Agent &You are looking for a restaurant is that right ?  \\
7 & Cust &Yes.  \\
8 & Agent &Prezzo is a nice restaurant in the west of town serving italian food.  \\
9 & Cust &What is the phone number ?  \\
10 & Agent &The phone number of prezzo is 097 6567 865.  \\
11 & Cust & Goodbye.  \\
\hline\hline
12 & \multicolumn{2}{l|}{{\bf What is Food ? Answer: Italian - Supporting Fact : 3}} \\
\hline
\end{tabular}
\label{tab:food}
\end{table}

\begin{table}[ht!]
\centering
\caption{{\bf One supporting fact task} : A machine reading task formulated dialog state tracking learning example for the {\it Area} slot from  {\it DSTC2} dataset}
\begin{tabular}{|l|l|l|}
\hline
{\bf Index} & {\bf Actor} & {\bf Utterance} \\
\hline\hline
1 & Cust& I'm looking for italian food. \\
2 & Agent & Would you like something in the cheap moderate or expensive price range ? \\
3 & Cust& Moderate. \\
4 & Agent& What part of town do you have in mind ? \\
5 & Cust& North. \\
6 & Agent& Sorry there is no moderate restaurant in the north of town serving italian food. \\
7 & Cust & Thank you good bye. \\
\hline\hline
8 & \multicolumn{2}{l|}{{\bf What is Area ? Answer: North - Supporting Fact : 5}} \\
\hline
\end{tabular}
\label{tab:area}
\end{table}

\begin{table}[ht!]
\centering
\caption{{\bf One supporting fact task} : A machine reading task formulated dialog state tracking learning example for the {\it Pricerange} slot from {\it DSTC2} dataset}
\begin{tabular}{|l|l|l|}
\hline
{\bf Index} & {\bf Actor} & {\bf Utterance} \\
\hline\hline
1 &Cust &What kind of restaurant that serves french food. \\
2 &Agent &Restaurant two two serves french food. \\
3 &Cust &I dont care about the price range with the address. \\
4 &Agent &Sure restaurant two two is on chesterton road chesterton. \\
5 &Cust &Thank you goodbye. \\
\hline\hline
6 &  \multicolumn{2}{l|}{{\bf What is Pricerange? Answer: Dontcare - Supporting Fact : 3}} \\
\hline
\end{tabular}
\label{tab:price}
\end{table}

\begin{table}[ht!]
\centering
\caption{{\bf Yes-No question task} : A machine reading task formulated dialog state tracking learning example for the {\it Area} slot from  {\it DSTC2} dataset}
\begin{tabular}{|l|l|l|}
\hline
{\bf Index} & {\bf Actor} & {\bf Utterance} \\
\hline\hline
1 &Cust & I need a moderately priced north part of town. \\
2 &Agent & You are looking for a restaurant is that right. \\
3 &Cust &Yes. \\
4 &Agent & Golden wok is a nice restaurant in the north of town in the moderate price range. \\
5 &Cust &What is the address and phone number of. \\
6 &Agent& The phone number of golden wok is 987 678 65 and it is on histon road chesterton. \\
7 &Cust & Thank you good bye. \\
\hline
8 &\multicolumn{2}{l|}{{\bf Is area north ? Answer: Yes - Supporting Fact : 1}}\\
\hline
\end{tabular}
\label{tab:yesno}
\end{table}

\begin{table}[ht!]
\centering
\caption{{\bf Indefinite knowledge task} : A machine reading task formulated dialog state tracking learning example for the {\it Food} slot from  {\it DSTC2} dataset}
\begin{tabular}{|l|l|l|}
\hline
{\bf Index} & {\bf Actor} & {\bf Utterance} \\
\hline\hline
1 &Cust& I'm looking for a cheap restaurant in north.\\
2 &Agent& The royal spice is a nice restaurant in the north of town in the cheap price range.\\
3 &Cust& I would like the phone number.\\
4 &Agent& The phone number of royal spice is  987 678 65.\\
5 &Cust& Thank you goodbye.\\
\hline
6 & \multicolumn{2}{l|}{{\bf Is food Indian ? Maybe - Supporting Fact : 1}} \\
\hline
\end{tabular}
\label{tab:ik}
\end{table}

\begin{table}[ht!]
\centering
\caption{{\bf Counting task} : A machine reading task formulated dialog state tracking learning example for the {\it Food} slot from {\it DSTC2} dataset}
\begin{tabular}{|l|l|l|}
\hline
{\bf Index} & {\bf Actor} & {\bf Utterance} \\
\hline\hline
1 & cust&  I'd like a portuguese or brazilian restaurant. \\
2 & Agent&  Nandos city centre serves portuguese food. \\
3 & Cust&  What is the address. \\
4 & Agent&  sure nandos city centre is on 17 - saint andrews street. \\
5 & Cust&  Thank you good bye. \\
\hline
6 & \multicolumn{2}{l|}{{\bf How many food ? Answer: Two - Supporting Fact : 1}} \\
\hline
\end{tabular}
\label{tab:ct}
\end{table}

\begin{table}[ht!]
\centering
\caption{{\bf Listing task} : A machine reading task formulated dialog state tracking learning example for the {\it Area} slot from {\it DSTC2} dataset}
\begin{tabular}{|l|l|l|}
\hline
{\bf Index} & {\bf Actor} & {\bf Utterance} \\
\hline\hline
1 &Cust & Im looking for a cheap restaurant in the west or east part of town. \\
2 &Agent& Thanh Binh is a nice restaurant in the west of town in the cheap price range. \\
3 &Cust &What is the address and post code. \\
4 &Agent &Thanh Binh is on magdalene street city centre.\\
5 &Cust &Thank you goodbye.  \\
\hline
6 &  \multicolumn{2}{l|}{{\bf What is area ? Answer: \{West,East\} - Supporting Fact : 1}} \\
\hline
\end{tabular}
\label{tab:list}
\end{table}

\begin{table}[ht!]
\small
\centering
\caption{Attention shifting example for the {\it PriceRange} slot from {\it DSTC2} dataset}
\begin{tabular}{|l|l|l|l|l|l|l|}
\hline
{\bf Actor } & {\bf Utterance }& {\bf Hop 1 } & {\bf Hop 2 } & {\bf Hop 3 } & {\bf Hop 4 } & {\bf Hop 5 } \\
\hline
Cust& Im looking for a cheap restaurant that serves chinese food	&0.00	&\cellcolor{blue!14}0.14	&\cellcolor{blue!1}0.01	&0.00	&0.00 \\
\hline
Agent& What part of town do you have in mind	&\cellcolor{blue!2}0.02	&\cellcolor{blue!17}0.17	&\cellcolor{blue!5}0.05	&0.00	&0.00 \\
\hline
Cust& I dont care	&0.00	&0.00	&\cellcolor{blue!14}0.14	&0.00	&0.00 \\
\hline
Agent& Rice house serves chinese food in the cheap price range	&0.00&	\cellcolor{blue!2}0.02	&\cellcolor{blue!3}0.03&	\cellcolor{blue!98}0.98	&\cellcolor{blue!100}1.00 \\
\hline
Cust& What is the address and telephone number	&\cellcolor{blue!57}0.57  &\cellcolor{blue!7}0.07&	 \cellcolor{blue!15}0.15	&0.00	&0.00 \\
\hline
Agent& Sure rice house is on mill road city centre	& \cellcolor{blue!3}0.03 &	\cellcolor{blue!1}0.01	& \cellcolor{blue!13}0.13& \cellcolor{blue!2}	0.02	&0.00 \\
\hline
Cust& Phone number	&0.00	&\cellcolor{blue!1}0.01&	\cellcolor{blue!3}0.03	&0.00	&0.00 \\
\hline
Agent& The phone number of rice house is  765-239-09	& \cellcolor{blue!37} 0.37	&\cellcolor{blue!58}0.58&	\cellcolor{blue!45}0.45	&0.00	&0.00 \\
\hline
Cust& Thank you good bye	&0.00&	0.00	&0.00	&0.00	&0.00 \\
\hline
\multicolumn{7}{|l|}{{\bf What is the pricerange ? Answer: cheap}} \\
\hline
\end{tabular}
\label{tab:mem1}
\end{table}

\begin{table}[ht!]
\small
\centering
\caption{Attention shifting example for the {\it Food} slot from {\it DSTC2} dataset}
\begin{tabular}{|l|l|l|l|l|l|l|}
\hline
{\bf Actor } & {\bf Utterance }& {\bf Hop 1 } & {\bf Hop 2 } & {\bf Hop 3 } & {\bf Hop 4 } & {\bf Hop 5 } \\
\hline
Cust& The restaurant in any area that serves japanese food	&\cellcolor{blue!1}0.01	&0.00&	\cellcolor{blue!27}0.27	&\cellcolor{blue!100}1.00&	\cellcolor{blue!100}1.00  \\
\hline
Agent& \begin{tabular}{@{}l@{}} wagamama is a nice restaurant in the centre of town \\ serving japanese food \end{tabular} &	\cellcolor{blue!95}0.95&	\cellcolor{blue!100}1.00&	\cellcolor{blue!73}0.73	&0.00	&0.00  \\ 
\hline
Cust& Phone number&	0.00	&0.00	&0.00&	0.00	&0.00  \\
\hline
Agent& Can i help you with anything else	&0.00&	0.00&	0.00	&0.00	&0.00  \\
\hline
Cust& What is the phone number	&\cellcolor{blue!4}0.04&	0.00	&0.00&	0.00&	0.00  \\
\hline
Agent& The phone number of wagamama is 987-765-67	&0.00	&0.00&	0.00	&0.00&	0.00  \\
\hline
Cust& Thank you goodbye&	0.00&	0.00	&0.00&	0.00&	0.00  \\
\hline
\multicolumn{7}{|l|}{{\bf What is the food type ? Answer: japanese}} \\
\hline
\end{tabular}
\label{tab:mem2}
\end{table}

\begin{table}[ht!]
\small
\centering
\caption{Attention shifting example for the {\it Area} slot from {\it DSTC2} dataset}
\begin{tabular}{|l|l|l|l|l|l|l|}
\hline
{\bf Actor } & {\bf Utterance }& {\bf Hop 1 } & {\bf Hop 2 } & {\bf Hop 3 } & {\bf Hop 4 } & {\bf Hop 5 } \\
\hline
Cust& Im looking for a cheap restaurant that serves chinese food	&0.00	&\cellcolor{blue!18}0.18	&0.11	&0.04&	0.00 \\
\hline
Agent& What part of town do you have in mind	&\cellcolor{blue!33}0.33	&\cellcolor{blue!30}0.30&	0.00	&0.00&	0.00 \\
\hline
Cust& I dont care	&0.00	&0.00&	\cellcolor{blue!17}0.17	&\cellcolor{blue!37}0.37&	\cellcolor{blue!100}1.00 \\
\hline
Agent& Rice house serves chinese food in the cheap price range&	\cellcolor{blue!1}0.01	&0.00	&0.00	&0.00&	0.00 \\
\hline
Cust& What is the address and telephone number	&\cellcolor{blue!58}0.58	&\cellcolor{blue!9}0.09&	\cellcolor{blue!1}0.01	&0.00	&0.00 \\
\hline
Agent& Sure rice house is on mill road city centre	&\cellcolor{blue!3}0.03	&0.00	&0.00&	0.00&	0.00 \\
\hline
Cust& Phone number	&0.00&0.00&	0.00&	0.00&	0.00 \\
\hline
Agent& The phone number of rice house is 765-239-09	&\cellcolor{blue!2}0.02&	\cellcolor{blue!1}0.01&	0.00&	0.00	&0.00 \\
\hline
Cust& Thank you good bye	&\cellcolor{blue!2}0.02&	\cellcolor{blue!42}0.42	&\cellcolor{blue!71}0.71	&\cellcolor{blue!59}0.59&	0.00 \\
\hline
\multicolumn{7}{|l|}{{\bf What is the area ? Answer: dontcare}} \\
\hline
\end{tabular}
\label{tab:mem3}
\end{table}

%%%%%%%%%%%%%%%

\newpage
\section{Appendix}

\begin{table}[ht!]
\centering
\caption{{\bf One supporting fact task} : A machine reading task formulated dialog state tracking learning example for the {\it Food} slot from {\it DSTC2} dataset}
\begin{tabular}{|l|l|l|}
\hline\hline
{\bf Index} & {\bf Actor} & {\bf Utterance} \\
\hline
1 & Cust &West part of town cuban food.  \\
2 & Agent &Sorry there is no cuban restaurant in the west of town.  \\
3 & Cust &Ok, do you have an Italian place ?  \\
4 & Agent &Prezzo is a nice restaurant in the west of town serving italian food.  \\
5 & Cust &Phone number.  \\
6 & Agent &You are looking for a restaurant is that right ?  \\
7 & Cust &Yes.  \\
8 & Agent &Prezzo is a nice restaurant in the west of town serving italian food.  \\
9 & Cust &What is the phone number ?  \\
10 & Agent &The phone number of prezzo is 097 6567 865.  \\
11 & Cust & Goodbye.  \\
\hline\hline
12 & \multicolumn{2}{l|}{{\bf What is Food ? Answer: Italian - Supporting Fact : 3}} \\
\hline
\end{tabular}
\label{tab:food}
\end{table}

\begin{table}[ht!]
\centering
\caption{{\bf One supporting fact task} : A machine reading task formulated dialog state tracking learning example for the {\it Area} slot from  {\it DSTC2} dataset}
\begin{tabular}{|l|l|l|}
\hline
{\bf Index} & {\bf Actor} & {\bf Utterance} \\
\hline\hline
1 & Cust& I'm looking for italian food. \\
2 & Agent & Would you like something in the cheap moderate or expensive price range ? \\
3 & Cust& Moderate. \\
4 & Agent& What part of town do you have in mind ? \\
5 & Cust& North. \\
6 & Agent& Sorry there is no moderate restaurant in the north of town serving italian food. \\
7 & Cust & Thank you good bye. \\
\hline\hline
8 & \multicolumn{2}{l|}{{\bf What is Area ? Answer: North - Supporting Fact : 5}} \\
\hline
\end{tabular}
\label{tab:area}
\end{table}

\begin{table}[ht!]
\centering
\caption{{\bf One supporting fact task} : A machine reading task formulated dialog state tracking learning example for the {\it Pricerange} slot from {\it DSTC2} dataset}
\begin{tabular}{|l|l|l|}
\hline
{\bf Index} & {\bf Actor} & {\bf Utterance} \\
\hline\hline
1 &Cust &What kind of restaurant that serves french food. \\
2 &Agent &Restaurant two two serves french food. \\
3 &Cust &I dont care about the price range with the address. \\
4 &Agent &Sure restaurant two two is on chesterton road chesterton. \\
5 &Cust &Thank you goodbye. \\
\hline\hline
6 &  \multicolumn{2}{l|}{{\bf What is Pricerange? Answer: Dontcare - Supporting Fact : 3}} \\
\hline
\end{tabular}
\label{tab:price}
\end{table}

\begin{table}[ht!]
\centering
\caption{{\bf Yes-No question task} : A machine reading task formulated dialog state tracking learning example for the {\it Area} slot from  {\it DSTC2} dataset}
\begin{tabular}{|l|l|l|}
\hline
{\bf Index} & {\bf Actor} & {\bf Utterance} \\
\hline\hline
1 &Cust & I need a moderately priced north part of town. \\
2 &Agent & You are looking for a restaurant is that right. \\
3 &Cust &Yes. \\
4 &Agent & Golden wok is a nice restaurant in the north of town in the moderate price range. \\
5 &Cust &What is the address and phone number of. \\
6 &Agent& The phone number of golden wok is 987 678 65 and it is on histon road chesterton. \\
7 &Cust & Thank you good bye. \\
\hline
8 &\multicolumn{2}{l|}{{\bf Is area north ? Answer: Yes - Supporting Fact : 1}}\\
\hline
\end{tabular}
\label{tab:yesno}
\end{table}

\begin{table}[ht!]
\centering
\caption{{\bf Indefinite knowledge task} : A machine reading task formulated dialog state tracking learning example for the {\it Food} slot from  {\it DSTC2} dataset}
\begin{tabular}{|l|l|l|}
\hline
{\bf Index} & {\bf Actor} & {\bf Utterance} \\
\hline\hline
1 &Cust& I'm looking for a cheap restaurant in north.\\
2 &Agent& The royal spice is a nice restaurant in the north of town in the cheap price range.\\
3 &Cust& I would like the phone number.\\
4 &Agent& The phone number of royal spice is  987 678 65.\\
5 &Cust& Thank you goodbye.\\
\hline
6 & \multicolumn{2}{l|}{{\bf Is food Indian ? Maybe - Supporting Fact : 1}} \\
\hline
\end{tabular}
\label{tab:ik}
\end{table}

\begin{table}[ht!]
\centering
\caption{{\bf Counting task} : A machine reading task formulated dialog state tracking learning example for the {\it Food} slot from {\it DSTC2} dataset}
\begin{tabular}{|l|l|l|}
\hline
{\bf Index} & {\bf Actor} & {\bf Utterance} \\
\hline\hline
1 & cust&  I'd like a portuguese or brazilian restaurant. \\
2 & Agent&  Nandos city centre serves portuguese food. \\
3 & Cust&  What is the address. \\
4 & Agent&  sure nandos city centre is on 17 - saint andrews street. \\
5 & Cust&  Thank you good bye. \\
\hline
6 & \multicolumn{2}{l|}{{\bf How many food ? Answer: Two - Supporting Fact : 1}} \\
\hline
\end{tabular}
\label{tab:ct}
\end{table}

\begin{table}[ht!]
\centering
\caption{{\bf Listing task} : A machine reading task formulated dialog state tracking learning example for the {\it Area} slot from {\it DSTC2} dataset}
\begin{tabular}{|l|l|l|}
\hline
{\bf Index} & {\bf Actor} & {\bf Utterance} \\
\hline\hline
1 &Cust & Im looking for a cheap restaurant in the west or east part of town. \\
2 &Agent& Thanh Binh is a nice restaurant in the west of town in the cheap price range. \\
3 &Cust &What is the address and post code. \\
4 &Agent &Thanh Binh is on magdalene street city centre.\\
5 &Cust &Thank you goodbye.  \\
\hline
6 &  \multicolumn{2}{l|}{{\bf What is area ? Answer: \{West,East\} - Supporting Fact : 1}} \\
\hline
\end{tabular}
\label{tab:list}
\end{table}

\begin{table}[ht!]
\small
\centering
\caption{Attention shifting example for the {\it PriceRange} slot from {\it DSTC2} dataset}
\begin{tabular}{|l|l|l|l|l|l|l|}
\hline
{\bf Actor } & {\bf Utterance }& {\bf Hop 1 } & {\bf Hop 2 } & {\bf Hop 3 } & {\bf Hop 4 } & {\bf Hop 5 } \\
\hline
Cust& Im looking for a cheap restaurant that serves chinese food	&0.00	&\cellcolor{blue!14}0.14	&\cellcolor{blue!1}0.01	&0.00	&0.00 \\
\hline
Agent& What part of town do you have in mind	&\cellcolor{blue!2}0.02	&\cellcolor{blue!17}0.17	&\cellcolor{blue!5}0.05	&0.00	&0.00 \\
\hline
Cust& I dont care	&0.00	&0.00	&\cellcolor{blue!14}0.14	&0.00	&0.00 \\
\hline
Agent& Rice house serves chinese food in the cheap price range	&0.00&	\cellcolor{blue!2}0.02	&\cellcolor{blue!3}0.03&	\cellcolor{blue!98}0.98	&\cellcolor{blue!100}1.00 \\
\hline
Cust& What is the address and telephone number	&\cellcolor{blue!57}0.57  &\cellcolor{blue!7}0.07&	 \cellcolor{blue!15}0.15	&0.00	&0.00 \\
\hline
Agent& Sure rice house is on mill road city centre	& \cellcolor{blue!3}0.03 &	\cellcolor{blue!1}0.01	& \cellcolor{blue!13}0.13& \cellcolor{blue!2}	0.02	&0.00 \\
\hline
Cust& Phone number	&0.00	&\cellcolor{blue!1}0.01&	\cellcolor{blue!3}0.03	&0.00	&0.00 \\
\hline
Agent& The phone number of rice house is  765-239-09	& \cellcolor{blue!37} 0.37	&\cellcolor{blue!58}0.58&	\cellcolor{blue!45}0.45	&0.00	&0.00 \\
\hline
Cust& Thank you good bye	&0.00&	0.00	&0.00	&0.00	&0.00 \\
\hline
\multicolumn{7}{|l|}{{\bf What is the pricerange ? Answer: cheap}} \\
\hline
\end{tabular}
\label{tab:mem1}
\end{table}

\begin{table}[ht!]
\small
\centering
\caption{Attention shifting example for the {\it Food} slot from {\it DSTC2} dataset}
\begin{tabular}{|l|l|l|l|l|l|l|}
\hline
{\bf Actor } & {\bf Utterance }& {\bf Hop 1 } & {\bf Hop 2 } & {\bf Hop 3 } & {\bf Hop 4 } & {\bf Hop 5 } \\
\hline
Cust& The restaurant in any area that serves japanese food	&\cellcolor{blue!1}0.01	&0.00&	\cellcolor{blue!27}0.27	&\cellcolor{blue!100}1.00&	\cellcolor{blue!100}1.00  \\
\hline
Agent& \begin{tabular}{@{}l@{}} wagamama is a nice restaurant in the centre of town \\ serving japanese food \end{tabular} &	\cellcolor{blue!95}0.95&	\cellcolor{blue!100}1.00&	\cellcolor{blue!73}0.73	&0.00	&0.00  \\ 
\hline
Cust& Phone number&	0.00	&0.00	&0.00&	0.00	&0.00  \\
\hline
Agent& Can i help you with anything else	&0.00&	0.00&	0.00	&0.00	&0.00  \\
\hline
Cust& What is the phone number	&\cellcolor{blue!4}0.04&	0.00	&0.00&	0.00&	0.00  \\
\hline
Agent& The phone number of wagamama is 987-765-67	&0.00	&0.00&	0.00	&0.00&	0.00  \\
\hline
Cust& Thank you goodbye&	0.00&	0.00	&0.00&	0.00&	0.00  \\
\hline
\multicolumn{7}{|l|}{{\bf What is the food type ? Answer: japanese}} \\
\hline
\end{tabular}
\label{tab:mem2}
\end{table}

\begin{table}[ht!]
\small
\centering
\caption{Attention shifting example for the {\it Area} slot from {\it DSTC2} dataset}
\begin{tabular}{|l|l|l|l|l|l|l|}
\hline
{\bf Actor } & {\bf Utterance }& {\bf Hop 1 } & {\bf Hop 2 } & {\bf Hop 3 } & {\bf Hop 4 } & {\bf Hop 5 } \\
\hline
Cust& Im looking for a cheap restaurant that serves chinese food	&0.00	&\cellcolor{blue!18}0.18	&0.11	&0.04&	0.00 \\
\hline
Agent& What part of town do you have in mind	&\cellcolor{blue!33}0.33	&\cellcolor{blue!30}0.30&	0.00	&0.00&	0.00 \\
\hline
Cust& I dont care	&0.00	&0.00&	\cellcolor{blue!17}0.17	&\cellcolor{blue!37}0.37&	\cellcolor{blue!100}1.00 \\
\hline
Agent& Rice house serves chinese food in the cheap price range&	\cellcolor{blue!1}0.01	&0.00	&0.00	&0.00&	0.00 \\
\hline
Cust& What is the address and telephone number	&\cellcolor{blue!58}0.58	&\cellcolor{blue!9}0.09&	\cellcolor{blue!1}0.01	&0.00	&0.00 \\
\hline
Agent& Sure rice house is on mill road city centre	&\cellcolor{blue!3}0.03	&0.00	&0.00&	0.00&	0.00 \\
\hline
Cust& Phone number	&0.00&0.00&	0.00&	0.00&	0.00 \\
\hline
Agent& The phone number of rice house is 765-239-09	&\cellcolor{blue!2}0.02&	\cellcolor{blue!1}0.01&	0.00&	0.00	&0.00 \\
\hline
Cust& Thank you good bye	&\cellcolor{blue!2}0.02&	\cellcolor{blue!42}0.42	&\cellcolor{blue!71}0.71	&\cellcolor{blue!59}0.59&	0.00 \\
\hline
\multicolumn{7}{|l|}{{\bf What is the area ? Answer: dontcare}} \\
\hline
\end{tabular}
\label{tab:mem3}
\end{table}
